# Supplementary material for: Bear the Query in Mind: Visual Grounding with Query-conditioned Convolution
Source: arXiv:2206.09114 source file (2022-06-22)
Supplement: Supplementary file 1 [file supplement.tex]

\section{Implementation details.}
Our textual encoder is initialized with pre-trained BERT-base. In our visual encoder, the backbone ResNet model is initialized with ResNet-50 and the visual transformer encoders are initialized with the encoder of pre-trained DETR. Each candidate kernel in QCM is also initialized with the pre-trained kernel parameters. 
Furthermore, a noise sampled from a Gaussian distribution $\mathcal{N}(\mu,\sigma^{2})$ is added to each candidate kernel where $\mu = 0$ and $\sigma = 10^{-3}$. 
The non-linear projection $\phi(\cdot)$ is a ReLU-activated 2-layer MLP. 
We apply QCM to ResNet's layer 2, 3, and 4, and freeze the first layer of ResNet to reduce computation without hurting much performance. For each input image, we apply the common image augmentation and resizing method in previous work \cite{deng2021transvg,yang2020improving} to get augmented $640\times{640}$ input image.

\paragraph{Dataset statistics}
\begin{table}
\centering
\begin{tabular}{lrrlr} % https://www.tablesgenerator.com/
\toprule
Dataset  & images & queries & split & queries per set \\
\midrule
RefCOCO  & 19,994  & 142,210 & train & 120,624 \\
 & & & val &10,834 \\
 & & & testA & 5,657 \\
 & & & testB & 5,095     \\
RefCOCO+ & 19,992  & 141,564 & train & 120,191 \\
 & & & val & 10,758 \\
 & & & testA & 5,726 \\
 & & & testB &  4,889 \\
RefCOCOg & 25,799  &  95,010  & train-g & 85,474 \\
 & & & val-g &  9,536 \\
  & & & train-u & 80,512  \\
  & & & val-u & 4,896  \\
  & & & test-u & 9,602  \\
\bottomrule
\end{tabular}
\caption{Dataset statistics. RefCOCO and RefCOCO+ are split into train, val, testA and testB sets where testA contains queries only about people whereas
testB contains queries about non-people objects. For RefCOCOg, '-g' means RefCOCOg-google which splits data into train and val set, and '-u' means RefCOCOg-umd which splits data into train, val and test set.}
\label{tab:datasets}
\end{table}
%We use a learning rate of $0.0002$, a batch size of 32, a weight decay of $10^{-4}$, and a step scheduler that shrinks the learning rate by a factor of 0.1 every 60 epochs. We use AdamW optimizer for all our experiments. We also freeze the first layer of ResNet to reduce computation without hurting much performance. We train our model for 90 epochs on RefCOCO and RefCOCOg, and 180 epochs for RefCOCO+. Note that for RefCOCOg, we report the scores of the models trained on RefCOCO. More implementation details can be found in our source code.

\section{Supplementary Qualitative Analysis}
\begin{table*}[t]
\centering
\begin{tabular}{llrr}
\toprule
Query 1 & Query 2 & VGQC w/ fusion & VGQC w/o fusion \\
\midrule
woman in red dress & woman & 0.3251 & 0.4037 \\
lady red & woman & 0.3345 & 0.5081 \\
woman in red dress & lady red & 0.0001 & 0.0106\\
woman in red dress & man in striped shirt on bike & 0.6117 & 0.3894 \\
woman in red dress & stripped shirt & 0.5794 & 0.2779\\
man in striped shirt on bike & stripped shirt & 0.0112 & 0.0286 \\
stripped shirt & striped shirt & 0.0052 & 0.0143 \\
man in striped shirt on bike & striped shirt & 0.0033 & 0.0025 \\
\bottomrule
\end{tabular}

\caption{The cosine distance of the aggregated kernels in the query-conditioned convolution block {\#10} from each other using the same image with different queries. Similar queries are closer to each other while queries with different semantic meanings are far away from each other.}
\label{tab:dynamic-kernel-eachother-full}
\end{table*}
\begin{table*}[t]
\centering
\begin{tabular}{l|rl|rl}
\toprule
\multirow{2}{*}{Queries}    & \multicolumn{2}{c}{VGQC w/ fusion} & \multicolumn{2}{c}{VGQC w/o fusion} \\
          & Distance    & Attention weights $(\times 10^{-2})$\    & Distance     & Attention weights $(\times 10^{-2})$   \\
\midrule
woman in red dress & 0.4123 & [ 8.25  8.02  3.00  5.51 75.23] 
& 0.1803 & [42.58 27.95  4.85 17.56  7.04]\\
lady red & 0.4236 & [ 7.77  7.29  2.67  5.38 76.90] 
& 0.2276 & [49.95 23.58  4.52 15.45  6.48]\\
woman & 0.0175 & [14.57 17.50 19.63 23.14 25.16] 
& 0.4638 & [ 5.79 82.70  1.02  7.23  3.24]\\
man in striped shirt on bike & 0.1904 & [47.95 10.32  8.40 19.80 13.53] & 0.4568 & [ 7.44 81.54  1.10  6.81  3.09]\\
stripped shirt & 0.1751 & [44.02  6.75  7.10 24.06 18.07] 
& 0.3321 & [11.77 62.63  1.96 19.94  3.68]\\
striped shirt & 0.2066 & [48.79  6.74  7.46 20.93 16.07] 
& 0.4230 & [ 8.70 75.98  1.15 11.62  2.52] \\
\bottomrule
\end{tabular}
\caption{The cosine distance from the aggregated kernels to the reference aggregated kernel in the query-conditioned convolution block {\#10} using the same image with different queries. The reference aggregated kernel is the unweighted average of the five candidate kernels. Aggregated kernels with and without activated attention are at different distances from the reference kernel.}
\label{tab:dynamic-kernel-reference-full}
\end{table*}
\begin{figure}[h]
  \centering
  \includegraphics[width=1.0\linewidth]{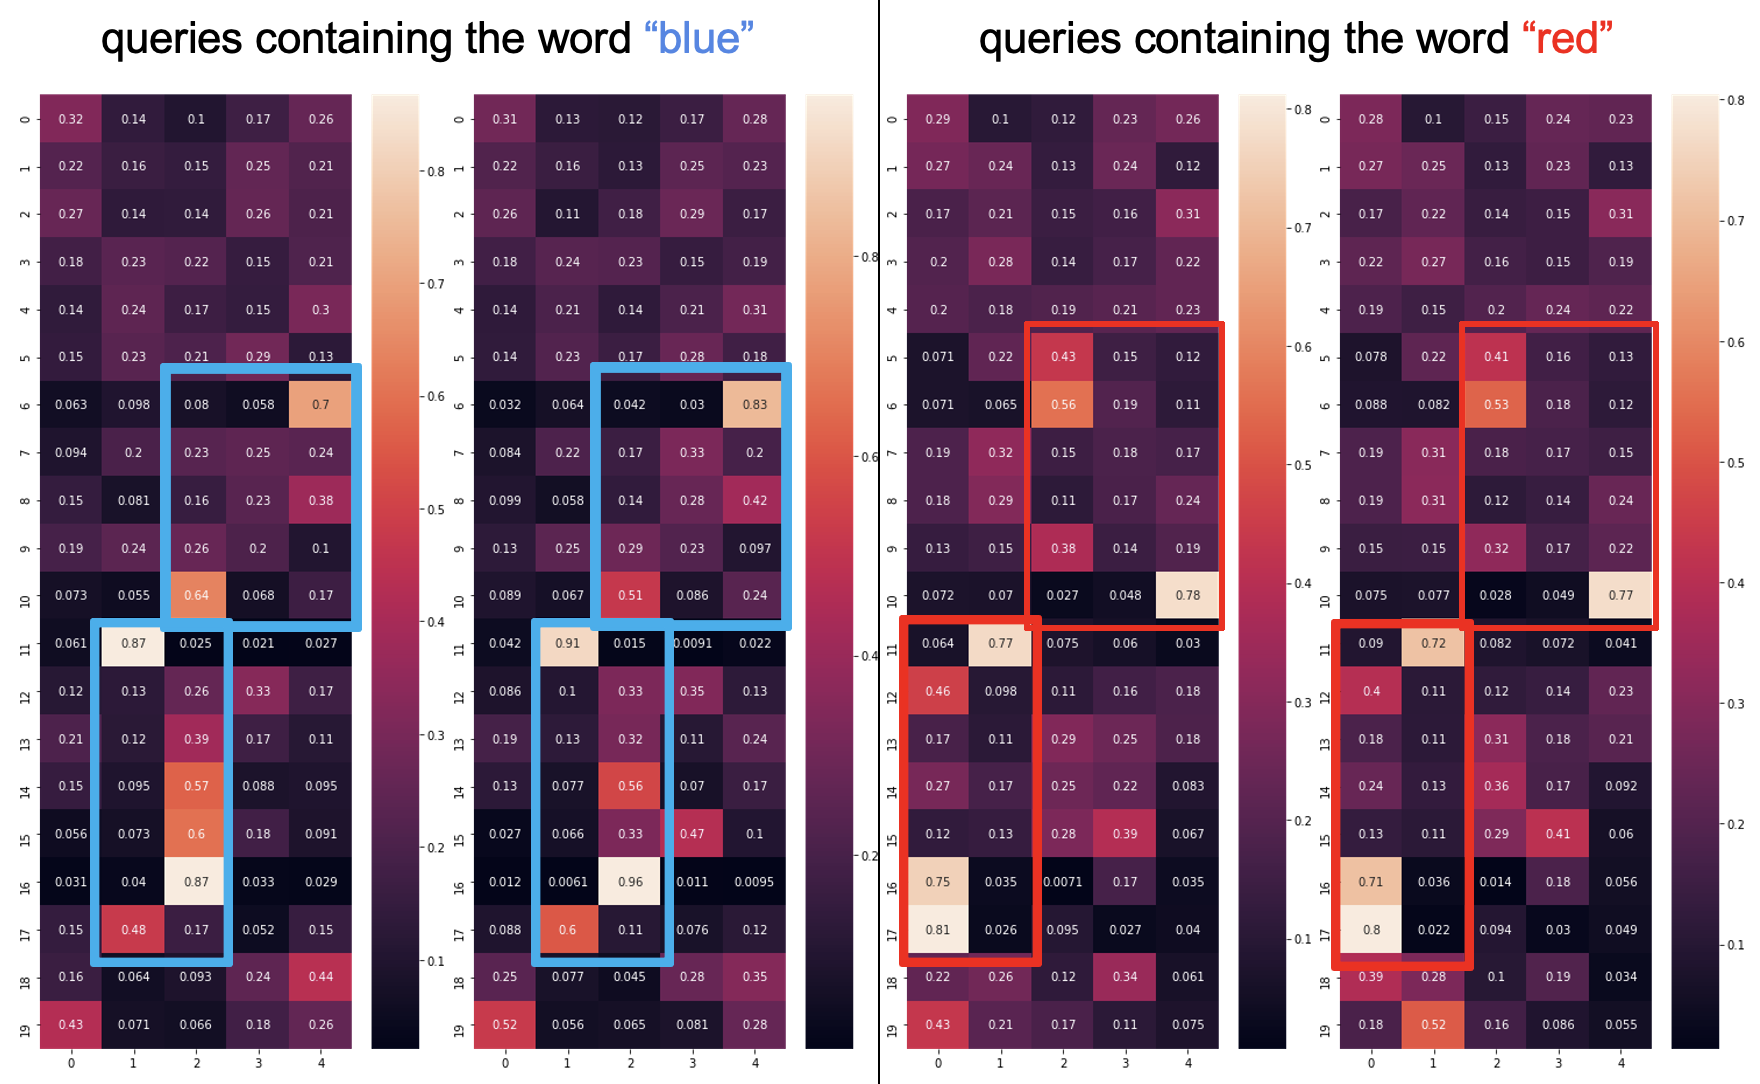}
  % \caption{Attention weights for all QCM blocks of VGQC w/ fusion model for four example queries shown at the top. Queries with similar meanings produce similar attention weights.}
  \caption{}%Attention weights for the last 4 out of 16 QCM blocks of VGQC w/ fusion model for 4 different queries shown at the top. $\alpha_k^{(i)}$ means the attention weight for $k$-th candidate kernel at block $i$.}
%   \oscar{20 blocks are a lot, and the attention weights in the lower part look good too.}
  \label{fig:supplement-attention-heatmap}
\end{figure}

\begin{table}[]
\centering
%\begin{tabular}{lrrrrrr}
%\toprule
%      & All & \#1 & \#2 & \#3 & \#4 & \#5  \\ \hline
%val   & 69.17 & 54.80    &  43.54   & 58.73    & 57.55    & 55.76     \\
%testA & 73.52 & 57.28    &  30.73   & 58.66    & 58.69    & 58.87     \\
%testB & 58.97 & 49.96    &  55.83   & 54.48    & 57.55    & 49.94      \\ \hline
%\end{tabular}

 \begin{tabular}{lrrrrrr}
 \toprule
      & All & Mean & -\#1 & -\#2 & -\#3 & -\#4 & -\#5  \\ \hline
 val  & 69.17 & 64.71 & 64.87 & 67.17 & 68.70 & 69.08 & 64.99  \\
 testA & 73.52 & 67.88 & 66.59 & 72.20 & 73.03 & 73.31 & 66.53  \\
 testB & 58.97 & 57.54 & 58.57 & 55.09 & 58.73 & 59.14 & 59.30 \\ \hline
 \end{tabular}
\caption{Overall accuracy (\%) on RefCOCO+ when VGQC w/ fusion masks one candidate kernel out in the final QCM block. For example, -\#2 means masking the second candidate kernel out. ``Mean" means using a fixed evenly-distributed attention. Their performances are worse than the normal VGQC w/ fusion model (column ``All"). % \chonghan{Is the second table necessary or can be removed?}
}

% \caption{Overall accuracy (\%) on RefCOCO+ when VGQC w/ fusion uses only one candidate kernel or masks one candidate kernel out in the final QCM block. For example, \#1 means using only the first candidate kernel, and -\#2 means masking the second candidate kernel out. ``Mean" means using a fixed evenly-distributed attention. Their performances are worse than the normal VGQC w/ fusion model (column ``All"). \chonghan{Is the second table necessary or can be removed?}}

\label{tab:candidate-kernel-ablation}
\end{table}

visualize our REG attention
