# Supplementary material for: Bear the Query in Mind: Visual Grounding with Query-conditioned Convolution
Source: arXiv:2206.09114 source file (2022-06-22)
Supplement: Supplementary file 2 [file supplement-attention-heatmap.tex]

\begin{figure}[h]
  \centering
  \includegraphics[width=1.0\linewidth]{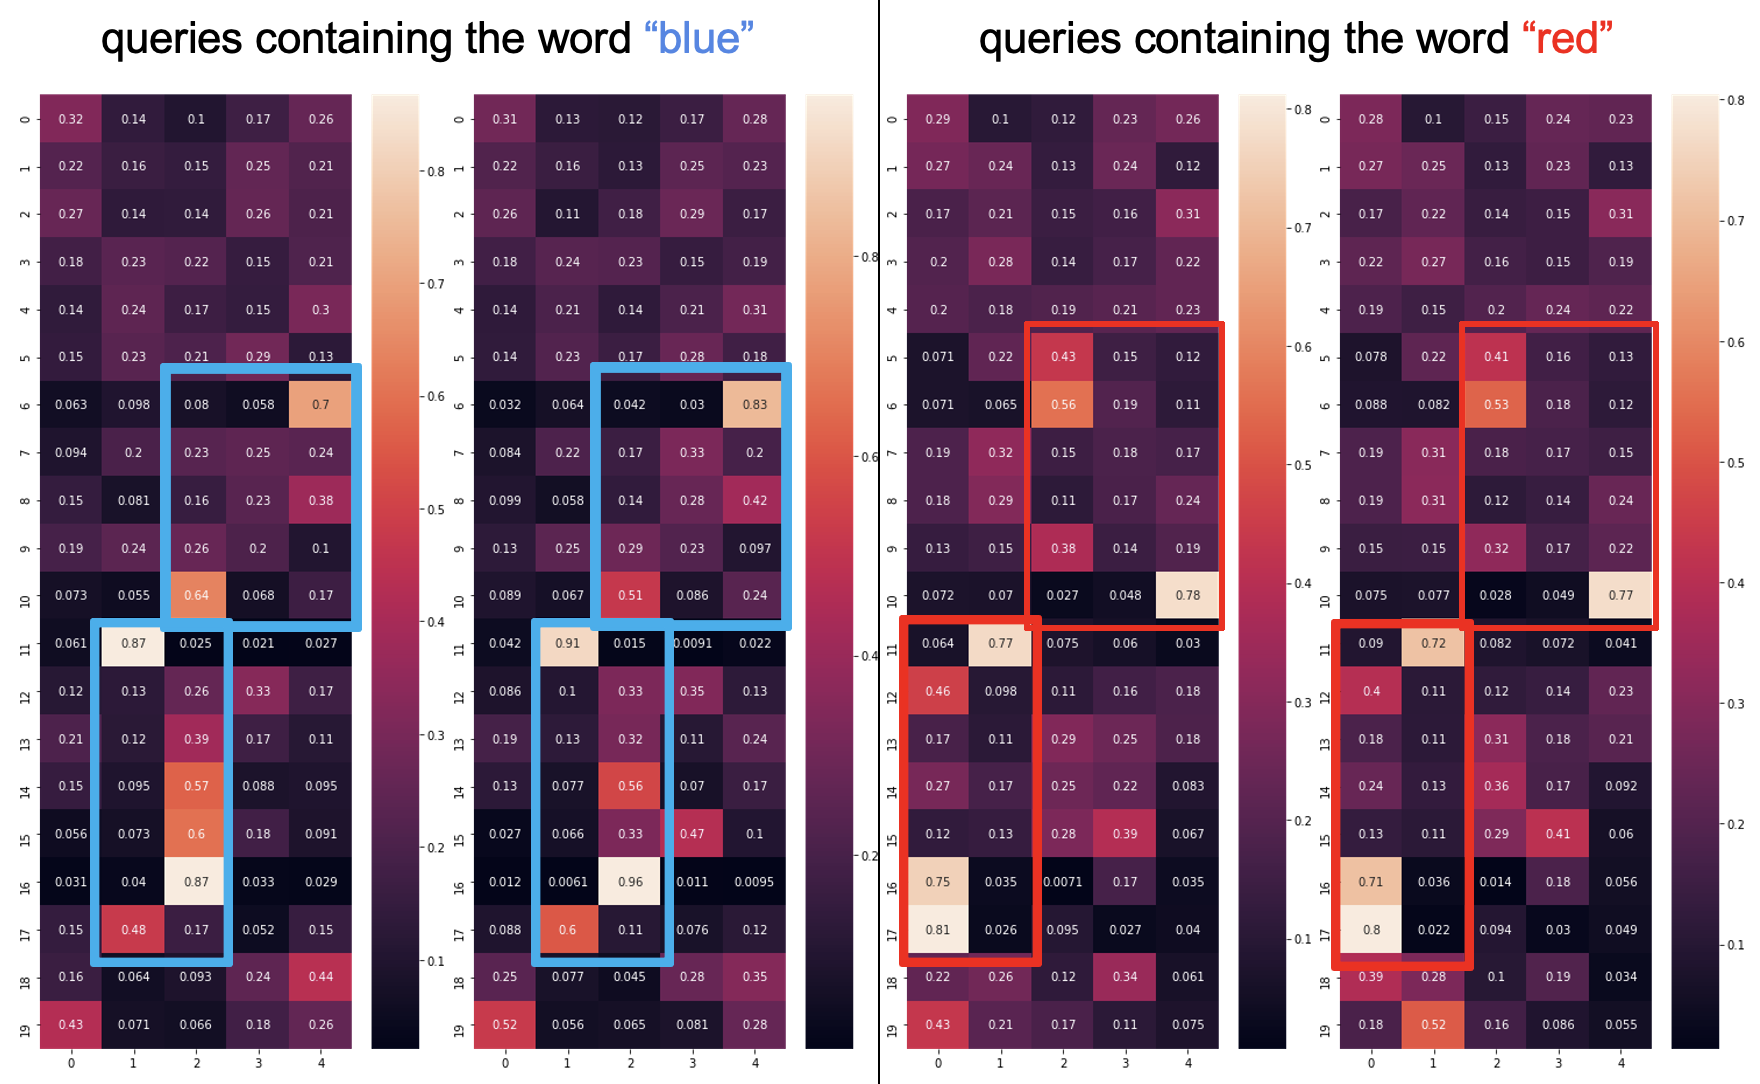}
  % \caption{Attention weights for all QCM blocks of VGQC w/ fusion model for four example queries shown at the top. Queries with similar meanings produce similar attention weights.}
  \caption{}%Attention weights for the last 4 out of 16 QCM blocks of VGQC w/ fusion model for 4 different queries shown at the top. $\alpha_k^{(i)}$ means the attention weight for $k$-th candidate kernel at block $i$.}
%   \oscar{20 blocks are a lot, and the attention weights in the lower part look good too.}
  \label{fig:supplement-attention-heatmap}
\end{figure}
