# Supplementary material for: Bear the Query in Mind: Visual Grounding with Query-conditioned Convolution
Source: arXiv:2206.09114 source file (2022-06-22)
Supplement: Supplementary file 3 [file supplement-candidatekernel-ablation.tex]

\begin{table}[]
\centering
%\begin{tabular}{lrrrrrr}
%\toprule
%      & All & \#1 & \#2 & \#3 & \#4 & \#5  \\ \hline
%val   & 69.17 & 54.80    &  43.54   & 58.73    & 57.55    & 55.76     \\
%testA & 73.52 & 57.28    &  30.73   & 58.66    & 58.69    & 58.87     \\
%testB & 58.97 & 49.96    &  55.83   & 54.48    & 57.55    & 49.94      \\ \hline
%\end{tabular}

 \begin{tabular}{lrrrrrr}
 \toprule
      & All & Mean & -\#1 & -\#2 & -\#3 & -\#4 & -\#5  \\ \hline
 val  & 69.17 & 64.71 & 64.87 & 67.17 & 68.70 & 69.08 & 64.99  \\
 testA & 73.52 & 67.88 & 66.59 & 72.20 & 73.03 & 73.31 & 66.53  \\
 testB & 58.97 & 57.54 & 58.57 & 55.09 & 58.73 & 59.14 & 59.30 \\ \hline
 \end{tabular}
\caption{Overall accuracy (\%) on RefCOCO+ when VGQC w/ fusion masks one candidate kernel out in the final QCM block. For example, -\#2 means masking the second candidate kernel out. ``Mean" means using a fixed evenly-distributed attention. Their performances are worse than the normal VGQC w/ fusion model (column ``All"). % \chonghan{Is the second table necessary or can be removed?}
}

% \caption{Overall accuracy (\%) on RefCOCO+ when VGQC w/ fusion uses only one candidate kernel or masks one candidate kernel out in the final QCM block. For example, \#1 means using only the first candidate kernel, and -\#2 means masking the second candidate kernel out. ``Mean" means using a fixed evenly-distributed attention. Their performances are worse than the normal VGQC w/ fusion model (column ``All"). \chonghan{Is the second table necessary or can be removed?}}

\label{tab:candidate-kernel-ablation}
\end{table}
